# Supplementary material for: The g2p Experiment: A Measurement of the Proton's Spin Structure Functions
Source: arXiv:1708.08297 source file (2017-08-25)
Supplement: Supplementary file 1 [file Appendix-B.tex]

\chapter{\sc Low Trigger Effiency Runs }
\label{app:Appendix-B}

%The 26 runs where the RHRS trigger efficiency falls below 99\% are shown in Figure~\ref{table:Problems}.
A run status of ``1" corresponds a production run and a run status of ``3" correspond to a dilution run in Table~\ref{table:Problems}.

\begin{table}[htp]
\begin{center}
\begin{tabular}{|c|c|c|c|c|}
\hline
Run Number & E0 (GeV) & P0 (GeV) & RunStatus & Eff\\ \hline
23685& 1.15 & 1.017 & 3& 98.88\\ \hline
23686& 1.15 & 1.017 & 3& 98.89\\ \hline
23687& 1.15 & 1.017 & 3& 98.92\\ \hline
23688& 1.15 & 1.017 & 3&98.94\\ \hline
23689& 1.15 & 1.017 & 3&98.96\\ \hline
23690& 1.15 & 1.017 & 3&98.97\\ \hline
23895& 1.15 & 1.081 & 1&98.86\\ \hline
23896& 1.15 & 1.081 & 1&98.85\\ \hline
23897& 1.15 & 1.081 & 1&98.88\\ \hline
23898& 1.15 & 1.081 & 1&98.88\\ \hline
23899& 1.15 & 1.081 & 1&98.86\\ \hline
23900& 1.15 & 1.081 & 1&98.86\\ \hline
23901& 1.15 & 1.081 & 1&98.86\\ \hline
23902& 1.15 & 1.081 & 1&98.93\\ \hline
23903& 1.15 & 1.081 & 1&98.89\\ \hline
23904& 1.15 & 1.081 & 1&98.89\\ \hline
24779& 3.35 & 1.945 &3&97.86\\ \hline
24780 & 3.35 & 1.945 &3&98.04\\ \hline
24781 & 3.35 & 1.945 &3&97.85\\ \hline
24788 & 3.35 & 1.945 &3&97.73\\ \hline
24789 & 3.35 & 1.945 &3&97.80\\ \hline
24790 & 3.35 & 1.945 &3&97.84\\ \hline
24791 & 3.35 & 1.945 &3&97.79\\ \hline
24792 & 3.35 & 1.945 &3&97.74\\ \hline
24793 & 3.35 & 1.945 &3&97.78\\ \hline
24794 & 3.35 & 1.945 &3&97.50\\ \hline
\end{tabular}
\end{center}
\caption{RHRS runs where the trigger efficiency falls below 99$\%$.}
\label{table:Problems}
\end{table}%
